# Supplementary material for: General Riemannian SOM
Source: arXiv:1505.03917 source file (2015-05-14)
Supplement: Supplementary file 1 [file appendix_euclidean_hex.tex]

\chapter{Appendix: Calculation of $a_{r,r'}, b_{r,r'}$ and their Fourier transforms}

\begin{eqnarray*}
 a_{r,r'} &=& \delta(r'-r) \matrixdrei{\frac 5 9 & 0 & 0\\ 0 & & 0 \\ 0 & 0& \frac 4 3 s^2} \\ 
	&-& \delta(r+e_x-r')  \matrixdrei{\frac 1 6  & 0 & 0 \\ - \frac 1 {3 \sqrt 3} & - \frac 1 {48} & 0 \\ 0 & 0 & - \frac 2 9 s^2} \\
	&-& \delta(r+e_x-r')  \matrixdrei{\frac 1 6  & 0 & 0 \\ + \frac 1 {3 \sqrt 3} & - \frac 1 {48} & 0 \\ 0 & 0 & - \frac 2 9 s^2} \\	
	&-& \delta(r+\frac {e_x}2 + \frac{\sqrt{3}}2 e_y-r')  \matrixdrei{\frac 1 {36}  & \frac 1 {9 \sqrt{3}} & 0 \\ () & () & 0 \\ 0 & 0 & - \frac 2 9 s^2} \\
	&-& \delta(r+\frac {e_x}2 - \frac{\sqrt{3}}2 e_y-r')  \matrixdrei{\frac 1 {36}  & - \frac 1 {9 \sqrt{3}} & 0 \\ -()  & ()  & 0 \\ 0 & 0 & - \frac 2 9 s^2} \\
	&-& \delta(r-\frac {e_x}2 + \frac{\sqrt{3}}2 e_y-r')  \matrixdrei{\frac 1 {36}  & - \frac 1 {9 \sqrt{3}} & 0 \\ -() & () & 0 \\ 0 & 0 & - \frac 2 9 s^2} \\
	&-& \delta(r-\frac {e_x}2 - \frac{\sqrt{3}}2 e_y-r')  \matrixdrei{\frac 1 {36}  & + \frac 1 {9 \sqrt{3}} & 0 \\ ()  & ()  & 0 \\ 0 & 0 & - \frac 2 9 s^2} 
\end{eqnarray*}

Calculating $\hat a(k)_{33}$:
\begin{eqnarray*}
 \hat a(k)_{33} &=&  \frac {4 s^2} 3- (e^ {i e_x k} + e^ {-i e_x k}) \frac {2 s^2} 9 \\
			&-& (e^ {i (\frac {e_x} 2 + \frac {\sqrt{3}} 2 e_y) k} +e^ {i (\frac {e_x} 2 - \frac {\sqrt{3}} 2 e_y) k} +e^ {i (-\frac {e_x} 2 + \frac {\sqrt{3}} 2 e_y) k} +e^ {-i (\frac {e_x} 2 + \frac {\sqrt{3}} 2 e_y) k}  ) \frac {2 s^2} 9\\
			&=&  \frac {4 s^2} 3 - \cos(k_x) \frac {2 s^2} 9 - \cos(\frac {k_x} 2 + \frac {\sqrt{3}} 2 k_y)  \frac {2 s^2} 9 -\cos(\frac {k_x} 2 - \frac {\sqrt{3}} 2 k_y) \frac {2 s^2} 9 \\
			&=&  \frac {4 s^2} 9 ( 3 - \cos(k_x) - \cos(\frac {k_x} 2 + \frac {\sqrt{3}} 2 k_y)  -\cos(\frac {k_x} 2 - \frac {\sqrt{3}} 2 k_y) 
\end{eqnarray*}

Calculating $\hat b(k)$:
\begin{eqnarray*}
\hat b(k) = f(k) e_x + g(k) e_y
\end{eqnarray*}

Calculating $\hat B_{33}$ (with long-ranged, gaussian $h$)
\begin{eqnarray*}
 \hat B_{33} &=& \frac {2 \pi \sigma^2}{N^2} (1 - \frac {4 s^2} 9 ( 3 - \cos(k_x) - \cos(\frac {k_x} 2 + \frac {\sqrt{3}} 2 k_y)  -\cos(\frac {k_x} 2 - \frac {\sqrt{3}} 2 k_y) ) e^{- \frac{k^2 \sigma^2} 2} )\\
		&=& \frac {2 \pi \sigma^2}{N^2} (1 - \frac {4 s^2} 9 ( 3 - (1- \frac{k_x^2} 2) - (1 - \frac {(\frac {k_x} 2 + \frac {\sqrt{3}} 2 k_y)^2} 2  - (1- \frac {(\frac {k_x} 2 - \frac {\sqrt{3}} 2 k_y)^2} 2) ) e^{- \frac{k^2 \sigma^2} 2} )\\
		&=& \frac {2 \pi \sigma^2}{N^2} (1 - \frac {4 s^2} 9 ( \frac {k^2_x} 2 + \frac {k^2_x} 4 +  \frac {3k^2_y} 4   ) e^{- \frac{k^2 \sigma^2} 2} )\\
		&=& \frac {2 \pi \sigma^2}{N^2} (1 - \frac {4s^2} 9 \frac {3k^2} 4  e^{- \frac{k^2 \sigma^2} 2} )\\
		&=& \frac {2 \pi \sigma^2}{N^2} (1 - \frac {s^2 k^2} 3  e^{- \frac{k^2 \sigma^2} 2} )
\end{eqnarray*}

Calculating eigenvalues of $\hat B$:
\begin{eqnarray*}
 \lambda^{\hat B}_3(k) &=&  \frac {2 \pi \sigma^2}{N^2} (1 - \frac {s^2 k^2} 3  e^{- \frac{k^2 \sigma^2} 2} )
\end{eqnarray*}
