# Supplementary material for: General Riemannian SOM
Source: arXiv:1505.03917 source file (2015-05-14)
Supplement: Supplementary file 2 [file generalized_SOM.tex]

\chapter{A Generalized View on Self Organizing Maps} \label{ch:gsom}

In this chapter, a generalization of the concept of Kohonen's self-organizing, topology preserving maps (SOM) will be discussed\footnote{For more details about the original algorithm see e.g. \cite{kohonen}, \cite[Ch.4]{ritter_schulten}}.
%Furthermore there will be an emphasis on the minimal properties of the map and the feature space, in which the SOM is working. Based on this view we will then derive a generalization of the original definition called \emph{General Riemannian SOM} (GR-SOM).

\section{The SOM Algorithm} \label{sec:som:algorithm}

First we will briefly introduce Kohonen's construction of the SOM. The SOM is a special kind of neural network where all neurons except certain input neurons lie in on single map layer. Thus every neuron is connected to the whole set of input fibers. From the neurophyiological point of view these are axons connected via synapses with the neurons. The strength of the connection is then given by a weight $w_{nl}$ for any synapse $l$ and neuron $n$. Furthermore are all the neurons interconnected so that excitations of certain neurons due to inputs can be propagate through the net of neurons, but can also be inhibited. Fig.\ref{fig:gsom:kfm} shows the corresponding formal network for the case of a two-dimensional input. For each input presented to the network the neurons then adapt themselves according to the Hebbian theory.\\

\begin{figure}[!ht]
\begin{center}
\includegraphics[width=0.42\linewidth]{../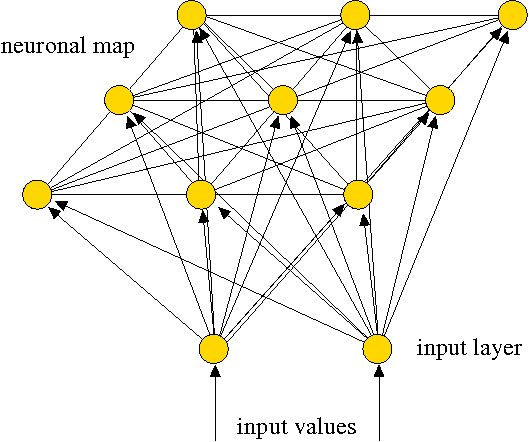}
\end{center}
\caption{formal Kohonen feature map with 2-dimenional input and 3x3 map}
\label{fig:gsom:kfm}
\end{figure}

To describe this process in detail a more mathematical approach is used. As an abstraction of this we can identify the input and the weights of each neuron $\vec w_n$ with vectors lying in a so-called \emph{feature space} $F$.
A self-organizing map is thereby a set $A$ of formal neurons $r$. Each of these per se abstract objects has then a \emph{representative} in the feature space according to the weights that we just mentioned. When data samples $v$ are presented in the feature space, the representative $w_r$ of the neurons will be adapted to represent the so given data set better. Motivated by the biological model there are also connections in the neuron layer allowing excitation of a neuron can be propagated to other neurons as well. In general this is modelled by the so-called \emph{neighborhood function} $h(r,s)$ that returns for each pair ($r$,$s$) of (distinct) neurons the strenth of the connection between them.\\
\\
Thus, the algorithm corresponding to the Hebb learning is given by:

\begin{enumerate}[Step 1:]

\item Initialize representatives of neurons with suitable values in $F$ e.g. random values.

\item Select a sample in $F$ according to sensoral input or a prespecified probability distribution.
\label{theo:SOM:alg_step2}

\item Determine winner neuron i.e. the neuron with the nearest representatives to the sample.
  \begin{equation} 
    \norm{w_s - v} = \min_{r \in A} \norm{w_r - v}
  \end{equation}

\item Adapt representatives in feature space:
   \begin{equation}
     w_r^{\mathrm{new}} = w_r^{\mathrm{old}} + \epsilon \cdot h(r,s) \cdot (v-w_r^{\mathrm{old}}) \quad \mathrm{for\ all\ } r\in A 
     \label{eqn:theo:SOM:adapt}
   \end{equation}
where $h^0(r,s)$ is the neighborhood function(see \ref{}) with values in $[0,1]$ and depending only on the distance of the neurons $r$ and $s$ in the map space and $\epsilon$ is the \emph{step size} parameter.

\item return to Step \ref{theo:SOM:alg_step2}

\end{enumerate}

%If using a prespecified probability distribution, these steps shape a Markov process of first order where the states are given by the ensemble of locations of the representatives $w_r$ in the feature space. The transition probability only depends on the present state and the prespecified distribution of the sample set $\set{v_i}$ in $F$.//
Regarding the choice of the winner neuron in the algorithm, each point in the feature space can be regarded to be attached to their particular winning neuron. Hence we get a voronoi tesselation of the feature space according to its metric (cf. Ch.\ref{sec:tess}). Each neuron is then a representative of a whole set of points namely all the points lying in the corresponding voronoi cell.

\section{Map space} \label{sec:som:mapspace}

 Taking another look at the biological model we will find that connections between the neurons will be stronger if they are in a certain way very close to each other (e.g. in respect to their distance in a grid). Analogously, the connection will be weaker otherwise or even inhibit the exitation of neurons that are farther away. This motivation is used in many mathemeatical approaches by defining a \emph{distance function} on the set of neurons, obtaining thus the structure of a \emph{metric space} and therefore a sense of ``closeness'' and neighbourhood (in the mathematical sense). The choice of the neighborhood function is then restricted to the case that it only depends on this distance rendering it translational invariant. We will denote the element of this subclass by $h^0$. In most cases the $h^0$ furthermore is monotonically decreasing and vanishes for larger distances corrensonding in the biological model to the fact that shorter connections are stronger than one that connect neurons lying at opposite side of the layer. Hence we get an adaption that is strongly lateral inhibited and so mostly local.\\
\\
Although at least our generalization of the feature space (cf. below) does not depend on this restriction of the neighborhood function, we have chosen to append this to our model of the GR-SOM by embedding the neurons into an additional space, the \emph{map space} $M$. There they are in contrast to the feature space all fixed. Then we model the lateral excitation by the neighboring function $h$ that was already used in the algorithm above and depends on the positions of the respective neurons relative to each other. A few examples for possible neighborhood functions will presented in a section further below. The fact that the adaption depend on the neighborhood function gives the SOM its most important feature that is the preservation of neighborhood. That means that neurons that are close in $M$, will also stay close to each other in the feature space.\\
Obviously, there are hardly any demands to the embedding space. That is that we need to be able to quantify the distance between two neurons in order to calculate the neighborhood function. Hence we must have at least a \emph{metric space}. In the numerical experiments we will mostly use Riemannian manifolds like the \emph{Euclidean Space} or the \emph{Hyperbolic Space}, but in general every set of points which has defined a metric on it can be used. The most simple one is the \emph{trivial space} i.e. a set of points associated with the discrete metric
\begin{eqnarray*}
 && d(x,x) = 0\\
 && d(x,y) = 1\quad \mathrm{if\ } x\neq y
\end{eqnarray*}
In this case however the topology is also the discrete topology and therefore each neighborhood. So its preservation IS trivial. Choosing a suitable neighborhood function, we just get a simple \emph{vector quantization}. Hence we see that we have to have pay at least a little bit attention to the choice of the metric.

\section{Feature space}

As in the map space the SOM algorithm directly demand a metric to be defined on the feature space. But in order to adapt the representatives, we furthermore need to determine how to move a point in direction to another one i.e. move the $w^{\mathrm{old}}_r$ towards the sample $v$. A suitable way is to move the point along the (geodesic) line between both points. A line is thereby, according to (Differential) Geometry (cf.e.g.\cite{aubin},\cite{abraham}), defined as a local length minimizing path. In general metric spaces the shortest path has not to be neither existent nor unique. So in order to stay consistent we have to put this restriction onto the used feature spaces. Fortunately this condition is always (at least) locally fulfilled by (pseudo-)Riemannian manifolds (cf.\cite[Thm.5.14]{aubin}). Thus to ensure that our modified adaption process that we will define below is always well-defined we restrict the possible choice of the feature space to those manifolds.

\section{General Riemannian SOM}

Taking the preceding two sections into consideration, we finally define our model of the \emph{General Riemannian SOM}. We thereby modify the classical SOM definition by adapting the algorithm in Eq.\ref{eqn:theo:SOM:adapt} to fit in the cases of the more general spaces. Hence we obtain:
\begin{equation}
 w_r^{\mathrm{new}} = p
\end{equation}
with $p \in F $ fulfilling the following conditions
\begin{equation}
d(w_r^{\mathrm{old}},p) + d(p,v) = d(w_r^{\mathrm{old}}, v), \frac {d(p,v)}  {d(p, w_r^{\mathrm{old}})} = \epsilon \cdot h^0(r,s)
\end{equation}
that means that the representative is moved along a geodesic between $ w_r^{\mathrm{old}}$ and $v$ by the relative distance according to the result of the neighborhood function and the step size. This adaption algorithm is well-defined as long as the geodesics are unique. According to the last section this will be the case for the right choice of the feature space. We will take a detailed look on this aspect with regard to the concrete spaces used in the simulations right in the next chapter. But before it, we will briefly take a look at the (classes of) neighborhood functions that will be used in the SOM.

\section{Neighbourhood functions} \label{sec:gsom:neighb_f}

As mentioned above, the SOM models itself to real neurons with their lateral inhibition of excitation. This inhibition is implemented by the neighborhood function. It depends only on distances in the mapspace and determines how extensive the adaption is. We can distinguished between three classes of possible functions:

\begin{description}

\item[Long range / Gaussian]

  One representative of the \emph{long-range} neighborhood functions is the \emph{Gaussian function} (with \emph{mean value} $\mu = 0$)

\begin{equation*}
  h^{Gauss}(x) = \frac 1 {\sqrt{2 \pi} \sigma} \exp(-\frac{x^2}{2 \sigma^2})
\end{equation*}
or in the case of a discrete grid of neurons
\begin{equation} \label{eqn:gsom:gauss}
  h^{Gauss}_{rr'} = \sum_s \delta_{r+s,r'} \exp(-\frac{s^2}{2 \sigma^2})
\end{equation}

where $sigma^2$ is the variance. With this class of function in use, the excitation is be lateral inhibited (i.e. $h$ is strictly decreasing), but has no upper limit for the range and thus affects the whole set of neurons. This results in an enormous need of computing time since in every step, each neuron has to be adapted.

\item[Short range / NN]

To evade the problem of the excessive needs  of the long-ranged functions in respect to computing time, the short-ranged functions possess an (bounded) compact support and therefore the excitation is locally restricted. Thus only a small fraction of the neurons has to be updated which accelerate the whole algorithm at the cost of losing interactions beyond the neighbourhood defined by support. An example for this family of functions is the following function:

\begin{equation} \label{eqn:gsom:NN}
  h^{NN}(x) = \Theta(x-d_{NN}) = \left\{ \begin{array}{ll} 1 & \mathrm{if\ neurons\ are\ nearest\ neighbors} \\  0 & \mathrm{otherwise} \end{array} \right. 
\end{equation}
where $d_{NN}$ is the distance of the nearest neighbors. We will consider this function besides the Gaussian one when working both numerically and analytically.

\item[Ultra-short range / VQ]

In the limit of small ranges and small variances both cases above lose their capability to assure the preservation of the neighborhood in the feature space. Only winner neurons are adapted, i.e. we have a case of \emph{vector quantization}.

\begin{equation}\label{eqn:gsom:vq}
  h^{VQ}(x) = \delta(x)
\end{equation}

\end{description}
