# Supplementary material for: General Riemannian SOM
Source: arXiv:1505.03917 source file (2015-05-14)
Supplement: Supplementary file 3 [file appendix_stability_hex.tex]

\subsection{Derivation in x}
